# Supplementary material for: Cost-aware Integration Process Modeling in Multiclouds
Source: arXiv:2103.08675 source file (2021-08-27)
Supplement: Supplementary file 1 [file appendix.tex]

\section{Realization and Design Decisions} \label{sec:realizaation}
% \todo[inline]{diagram and explanation for data gathering and processing? talk about stream and event architectures that the reviewers like}

Our approach is realized as shown in~\cref{fig:realization_approach}.
The pattern compositions and data specifications (incl. required capacities based on consumed main memory) from the SAP CPI standard content~\cite{sap-hci-content} are used to construct the IPCGs according to~\cite{DBLP:conf/debs/0001MFR18}.
Therefore the control and data flow of the compositions are reconstructed, and the integration content (incl. user-defined functions) is statically analyzed and annotated.
That means that the patterns are analyzed with respect to their shareability, and the resulting SH and CAP data (\ie from pattern benchmark~\cite{Ritter:2016:BIP:2933267.2933269}) are assigned resulting to extended IPCGs.

From there~\cref{fig:realization_approach} shows different optional processing variants.
% For a more fine-grained analysis of pattern compositions they can be pre-partitioned or \enquote{cut} according to the shareability property SH of their patterns.
% Essentially this means to increase the number of (sub-) compositions, while reducing their size to allow for a better fit during the platform assignment.
% Another optional step is to estimate a non-optimal, upper boundary of the number of required platform processing units (\eg by using bin packing) to constrain the search space.
While these graphs would already allow for an optimal partitioning of the complete compositions, we (a) conduct an optional pre-partitioning phase that \enquote{cuts} non-shareable sub-partitions out of else shareable compositions for comparison of the results, and (b) use techniques such as bin-packing to pre-calculate a better, but still non-optimal upper bound of the number of required containers.
Therefore platform cost models are assigned, taken from the market leading AWS\footnote{\url{https://aws.amazon.com/de/ec2/pricing/on-demand/}}, Microsoft Azure\footnote{\url{https://azure.microsoft.com/de-de/pricing/calculator/?service=container-service}}, and an anonymous platform $X$.
In addition, the tenant assignment of the pattern compositions is required for this and subsequent steps.

We briefly discuss our design decisions for the pre-processing in more detail along two hypotheses that are explained and evaluated subsequently.

\labeltitle{Tractability} %The problem for which we described an optimal solution is NP-complete.
%However, we study the practical tractability on real-world datasets with the goal to study the ...
\todo[inline]{move to heuristics section for motivation}
The latter (cf. (b)) targets an applicability study for the underlying theoretical problem is NP-hard (similar to~\cite{correia2008solving,jansen1999approximation}).
We argue that a pre-processing that reduces or restricts the search space is beneficial for a practical realization ($\rightarrow$ hypothesis \emph{HA}).
% bin-packing and sorting of container variants reduce the runtime in practice, by restricting the search space 
To evaluate HA, we developed a micro-benchmark that compares the runtime latencies of the optimal solution for an increasing number of pattern compositions from the C4C-CRM hybrid integration dataset of SAP CPI and one tenant using the open source GLPK v4.65\footnote{GNU Linear Programming Kit, visited 06/2020: \url{https://www.gnu.org/software/glpk/}} and CPLEX v12.8.0\footnote{IBM CPLEX, visited 06/2020: \url{https://www.ibm.com/analytics/cplex-optimizer}}), 
Thereby we applied bin-packing~\cite{zhang1997new} (not shown) and extra sorting constraints on the number of containers required for the solution $C$ according to their capacity $B_j$.
\begin{align*}
B_j \geq B_{j+1} && j \in [1,C[ \\
P_j \geq P_{j+1} && j \in [1,C[ 
\end{align*} %%%%\vspace{-.3cm}
The results are shown in~\cref{fig:latency}, which illustrates that the sorting slightly reduces the processing latency, because it removes many permutations of equal-cost variants in the search space, which further reduces the runtime.
\begin{figure}[bt]
	\centering
	\includegraphics[width=1\columnwidth]{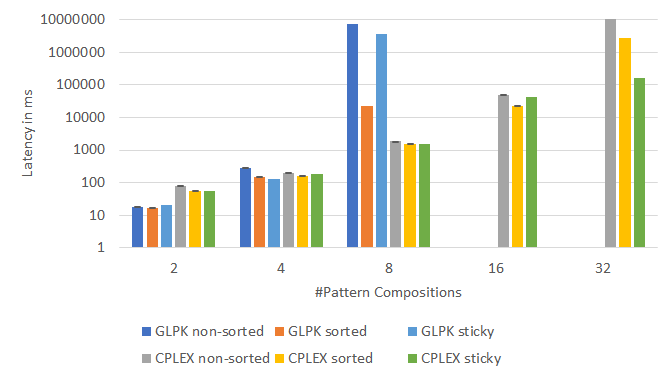}
	%%\vspace{-.7cm}
	\caption{CEPP solver benchmark}
	\label{fig:latency}
	%%\vspace{-0.3cm}
\end{figure}
The bin-packing is less beneficial smaller number of tenants, but together with the sorting, it keeps the stickiness (\ie customer preference not to share its compositions) to a minor impact on the solution processing.
For $32$ the combination of bin-packing and sorting improves the runtime, even with enabled stickiness. 
% stickiness has only a small impact (incl. pre-processing)
Furthermore, the GLPK solver is slightly faster than CPLEX only for small number of compositions up to eight.

\labeltitle{Design Decisions} In summary, we use the bin-packing with sorting in CPLEX configurations to face the complexity of the problem in a real-world context, according to hypothesis HA.
Furthermore following hypothesis HB, we use the correctness-preserving graph rewriting approach from~\cite{DBLP:conf/debs/0001MFR18} to pre-partition pattern compositions.

\section{Evaluation} \label{sec:evaluation}

\begin{figure}[ht]
	\centering
	\includegraphics[width=0.9\columnwidth]{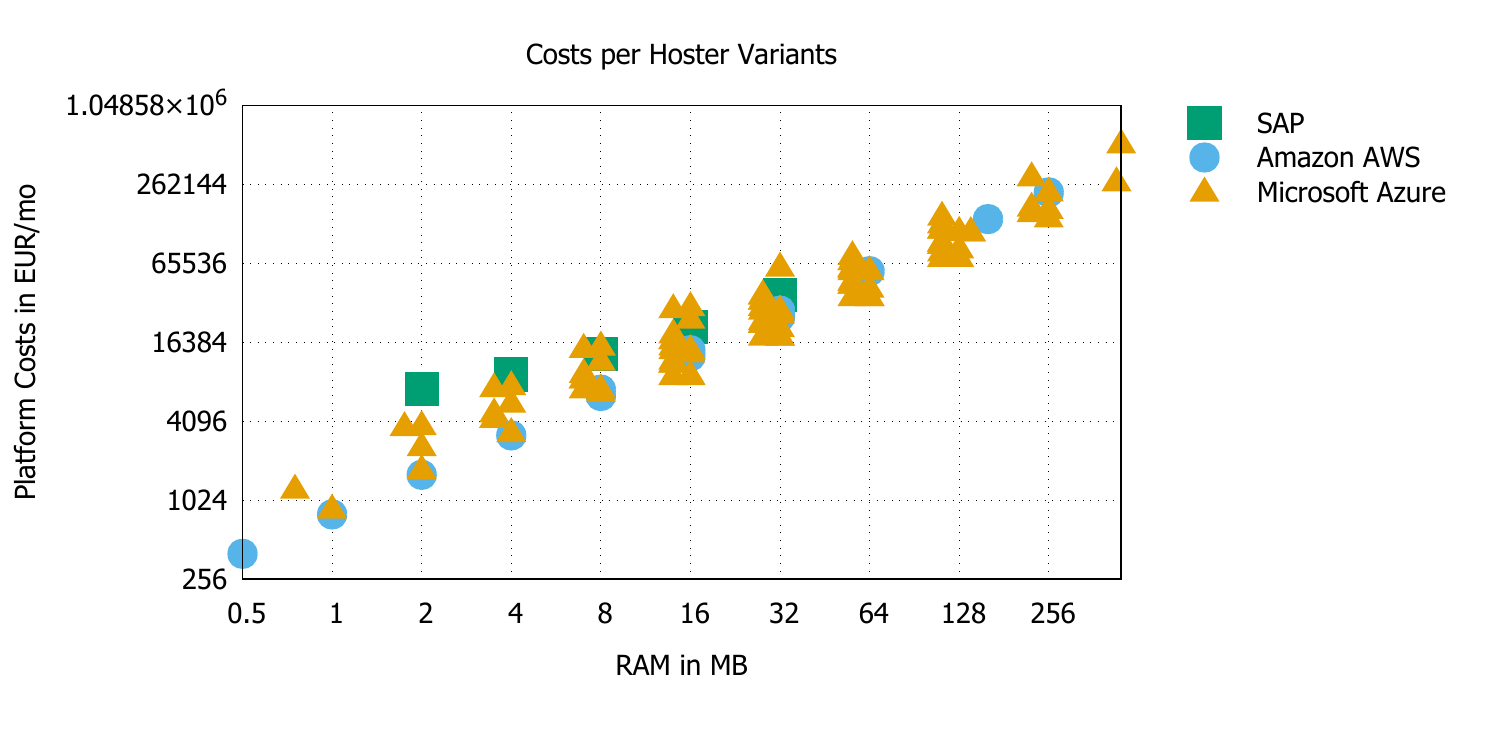} 
	\caption{Available container variants for IPCG partitioning}
	\label{fig:costModels}
\end{figure}

% \todo[inline]{introduce hypotheses linked to the research questions; make answers part of the case studies}
% In this section, we first share some details of our system realization and motivate our design choices based on experiments, before we conduct several case studies on real-world cloud integration data sets from SAP CPI to study the applicability of our approach based on two hypotheses that will be introduced subsequently.
In this section, we conduct several, quantitative case studies on real-world cloud integration data sets from SAP CPI to study the applicability of our approach based on several hypotheses that will be introduced subsequently.
We further qualitatively study the case of what we call \emph{Cost-driven Development} as a practical application of our approach.

In general, we assume that customer-specific hosting denotes the current state and allows for only one vendor and container, \ie 
\begin{itemize}
	\item all compositions are non-shareable,
	\item upper container bound equals to number of tenants,
	\item only one platform vendor cost model.
\end{itemize}
% denotes the current state.
From this customer-specific, one-container \enquote{hosting}, we set out to discuss the following hypotheses \emph{Hx} that target the INTaaS provider costs: %, that cost-wise not beneficial for the service provider compared to a
\begin{itemize}
	\item[H1] Multi-container is more beneficial than single-container hosting;
	\item[H2] A multicloud hosting is the most beneficial hosting variant (\ie leveraging different vendor cost models);
	%\end{itemize}
	%Further, we conjecture that
	%\begin{itemize}
	\item[H3] Multi-tenant shareability in a multicloud setup (\ie non-hosting) is beneficial for the INTaaS provider;
	\item[H4] Multi-tenant, multicloud setups can lead to trade-off: provider costs vs. customer latency;
	\item[H5] Security-aware pre-partitioning is beneficial for the INTaaS provider (follow-up from intermediate hypothesis HB in~\cref{sec:realizaation}).
\end{itemize}
% \todo[inline]{why no significant difference between H2 and H3 with respect to single-tenant setup}

To approach the trade-off one could add stickiness %(what is the effect of that?), 
or try to minimize the latency as subgoal to the costs under the following premise:
\begin{itemize}
	\item[H5] The latency subgoals increase the provider costs (not too drastically),
\end{itemize}
which could be granted for some customers or require increased costs.
Some customers have platform vendor preferences, which will increase the costs, and thus lead to an adaptation in the cost model for those cases, according to:
\begin{itemize}
	\item[H6] The provider costs increase significantly with vendor preferences of customers (maybe depending on the cost model strategy of the vendor).
\end{itemize}
Thereby we want to understand, whether vendors follow cost model strategies that make vendor preferences more severe for service providers:
\begin{itemize}
	\item[H7] Platform vendors follow certain cost model strategies.
\end{itemize}

\begin{example}[Motivating example (revisited)]
	When applying our approach to the motivating example, the optimal solution is a partitioning of the compositions to two containers from different vendors (AWS (30,00 EUR/mo), X (20,00 EUR/mo)) with cost $50.00$ EUR/mo, resulting to cost savings between 10.00 and 30.00 EUR/mo.
	%Two instead of three containers from two instead of one platform vendor selected.
	%Cost savings between 10.00 and 30.00 EUR per month with total costs of platform variant $AWS(30,00,1,6.25)$ as well as $X(20,00,1,3.125)$ result to costs of 50.00 EUR per month and full usage.
\end{example}

Already this simple example indicates that sharing pattern compositions over different platforms (\ie multicloud) can help to reduce costs for the INTaaS vendor (cf. H3).
Subsequently, we set out to give answers to these hypotheses through several case studies on real-world pattern compositions and costs.

\subsection{Case Studies: Cloud and Hybrid Integration}

We study the applicability and characteristics of our approach on real-world datasets and the impact of cutting original pattern compositions on the efficiency of the solution (cf. H1--H7).
While the studies only show the optimal costs for a small number of SAP CPI standard content~\cite{sap-hci-content} from 2016 and tenants --- due to the problem's complexity --- the cost saving potential becomes clearer, when putting the results into context to approximately 100+k compositions and 10+k tenants, currently on SAP CPI.

% Experiments:\\
% - test cut vs. un-cut compositions (very modular or not)\\
% - show stickiness\\
% - np problem, however, reducing the search space\\

% idea:\\
% - show that analysis of the content improves the number of containers required (Conclusions: for small number of tenants no impact, better for more tenants, however, these bin-packing results are not optimal for our case)\\
% - apply to differently classified content\\
% - standard content only\\
% - compare results for cost reduction and current vendors\\

%\begin{figure*}[tb]
%	\begin{center}$
%		\begin{array}{cc}
%		% runtime: 3,601,980 ms
%		\subfigure[Normal (costs=10,985 EUR/mo)]{\label{fig:c4c_normal_partitioning}\includegraphics[width=0.5\linewidth]{images/sap_crm_erp_three_tenants_no_cutting_sorting_binpacking_per_composition}} &
%		% runtime: 
%		\subfigure[Pre-Partitioned (costs=9,330 EUR/mo)]{\label{fig:c4c_pre-partitioned}\includegraphics[width=0.5\linewidth]{images/sap_crm_erp_three_tenants_with_cutting_sorting_binpacking_per_composition}}
%		\end{array}$
%	\end{center}
%	%%%%\vspace{-.5cm}
%	\caption{$x$ SAP C4C-CRM compositions from 2016 for three tenants (anonymized), \small with reference platform as X, Amazon Web Services as AWS, and Microsoft Azure (not selected); Format: \emph{platform}-\emph{costs/mo}-\emph{\#CPUs-RAM(GB)}}
%	\label{fig:}
%\end{figure*}

\begin{figure}[bt]
	\centering
	\includegraphics[width=1\columnwidth]{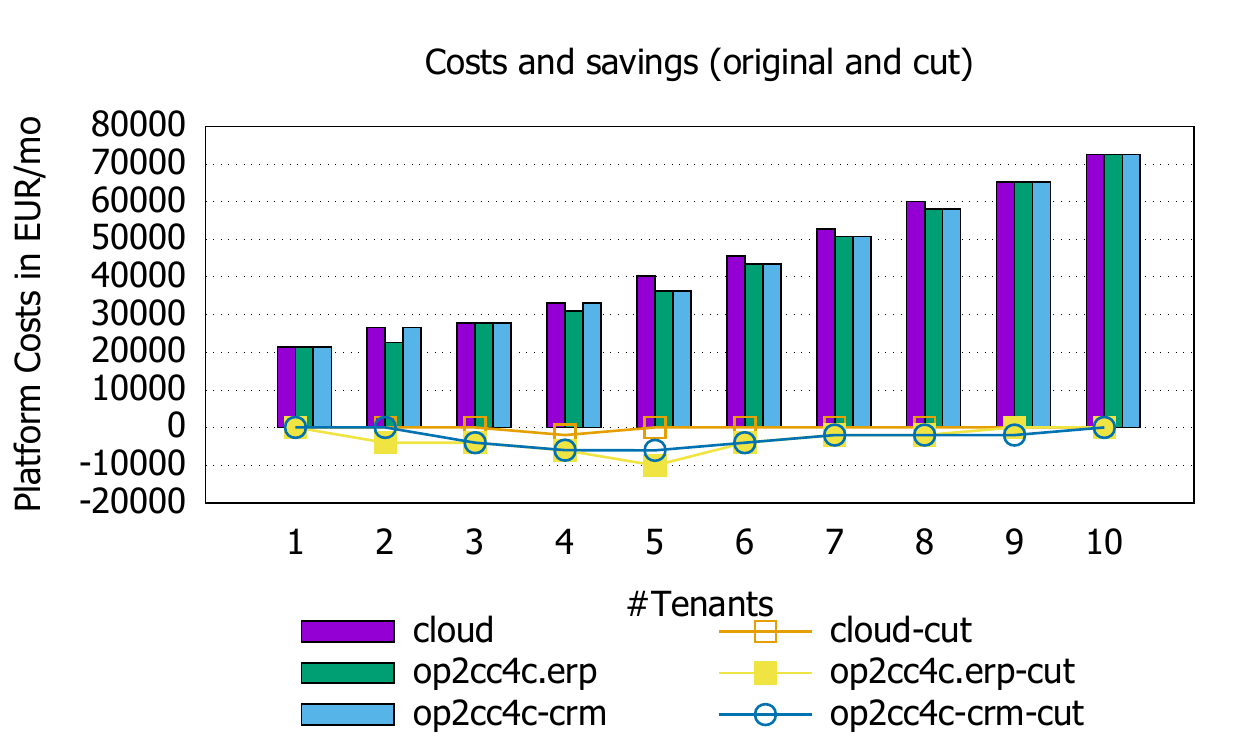}
	%%%\vspace{-.7cm}
	\caption{Current State (original and cut)}
	\label{fig:currentStateCut}
	%%%\vspace{-0.3cm}
\end{figure}

\begin{figure}[bt]
	\centering
	\includegraphics[width=1\columnwidth]{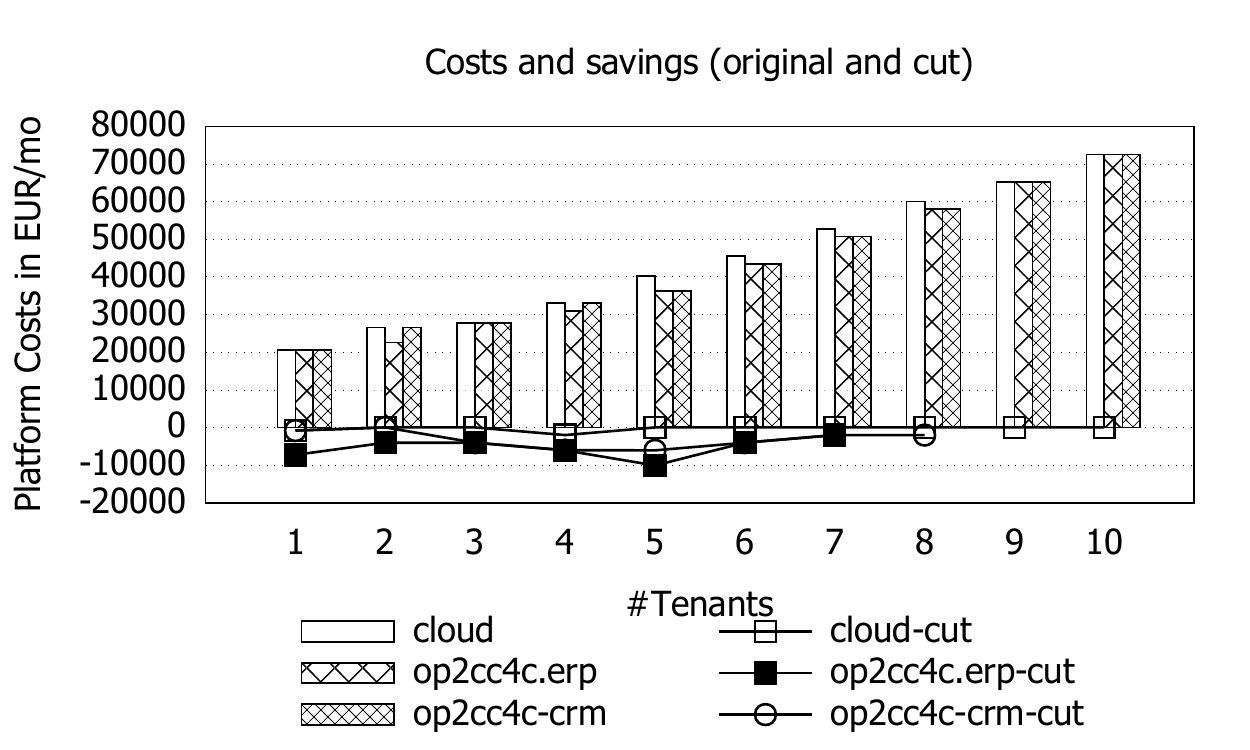}
	%%%\vspace{-.7cm}
	\caption{Hypothesis 1 (original and cut)}
	\label{fig:hypo1Cut}
	%%%\vspace{-0.3cm}
\end{figure}

\begin{figure}[bt]
	\centering
	\includegraphics[width=1\columnwidth]{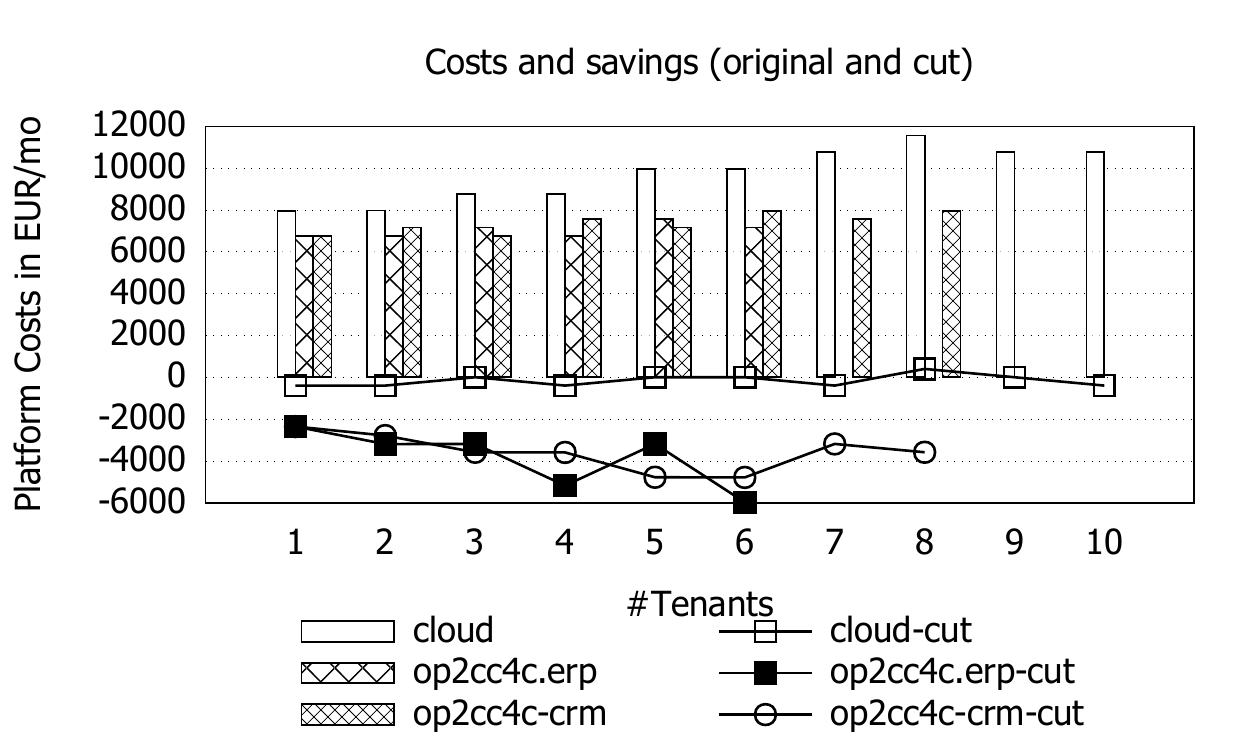}
	%%%\vspace{-.7cm}
	\caption{Hypothesis 2 (original and cut)}
	\label{fig:hypo2Cut}
	%%%\vspace{-0.3cm}
\end{figure}

\begin{figure}[bt]
	\centering
	\includegraphics[width=1\columnwidth]{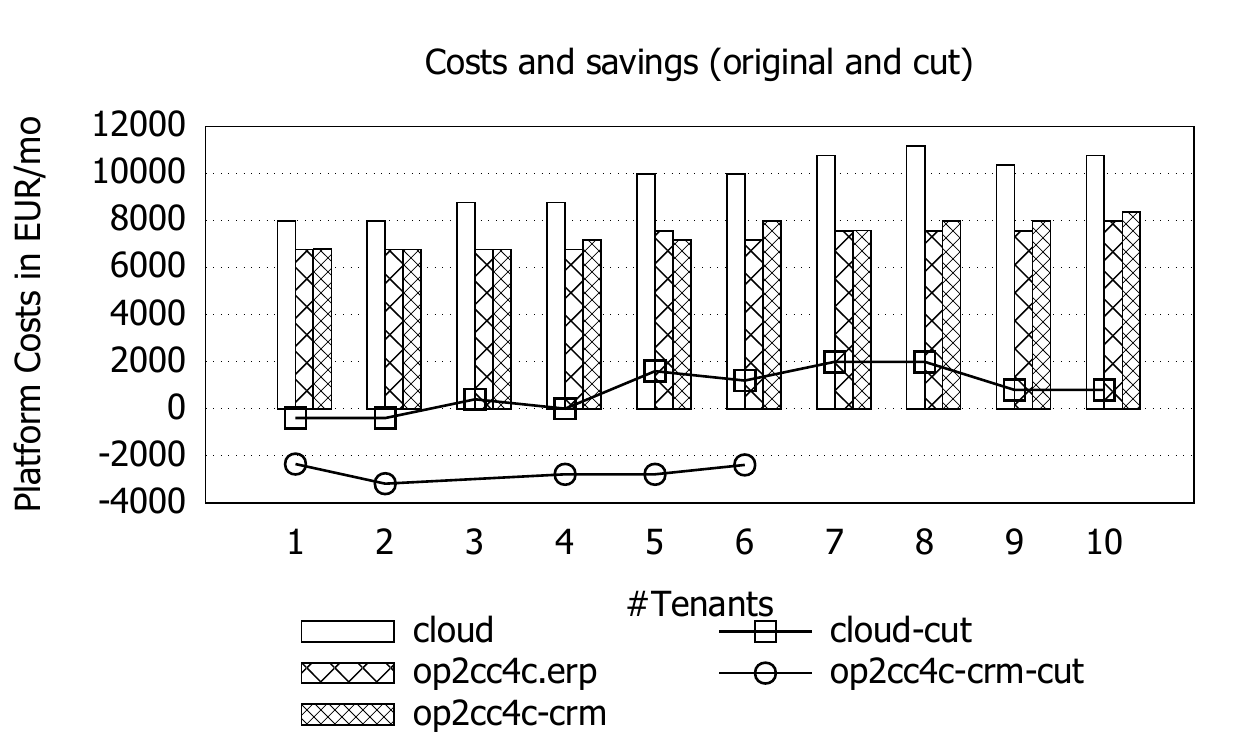}
	%%\vspace{-.7cm}
	\caption{Hypothesis 3 \& 4 (original and cut)}
	\label{fig:hypo3Cut}
	%%\vspace{-0.3cm}
\end{figure}

\begin{figure}[bt]
	\centering
	\includegraphics[width=1\columnwidth]{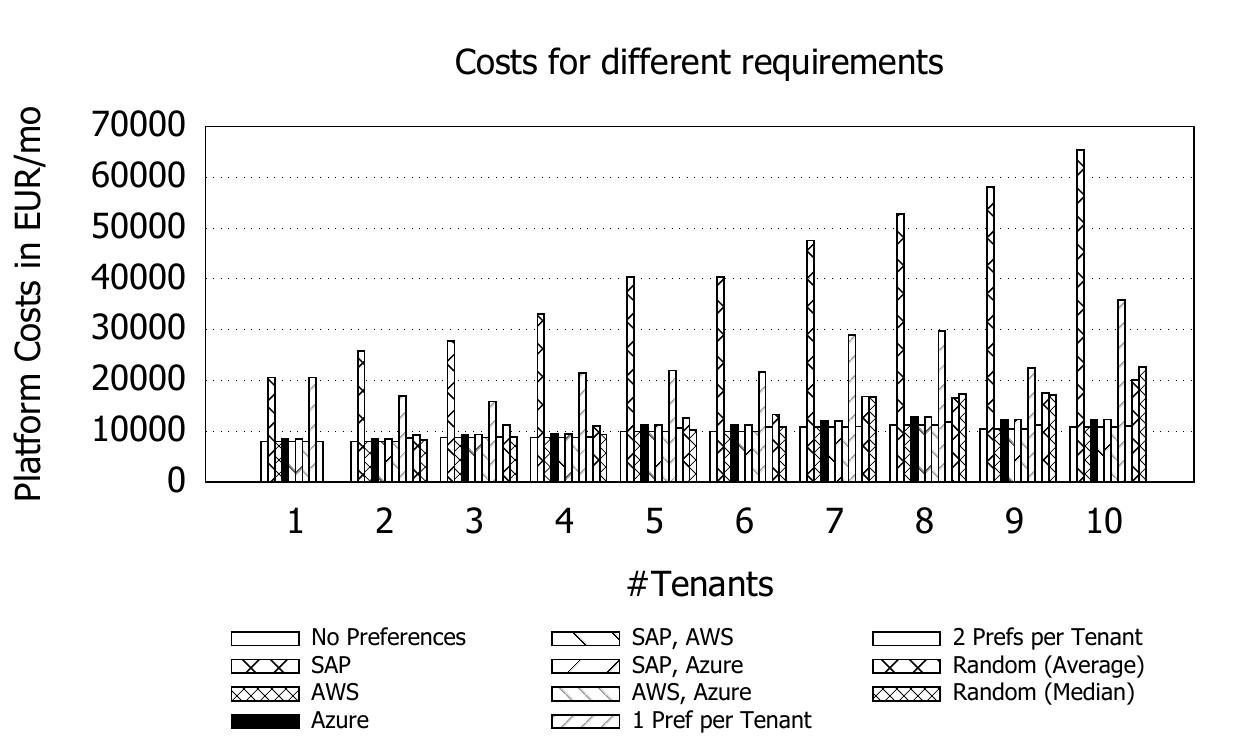}
	%%\vspace{-.7cm}
	\caption{Hypothesis 6 (with various preference distributions)}
	\label{fig:costModels}
	%%\vspace{-0.3cm}
\end{figure}

\labeltitle{Hypothesis 6} If the tenants have unconvenient preferences (e.g. only vendor X, or each tenant only one preference) the costs increase significantly. If th preferences are distributed randomly, the result becomes worse with increasing tenant number. The reason for this behaviour might be the increasing probability that at least one tenant has an expensive preference.

\begin{figure}[bt]
	\centering
	\includegraphics[width=1\columnwidth]{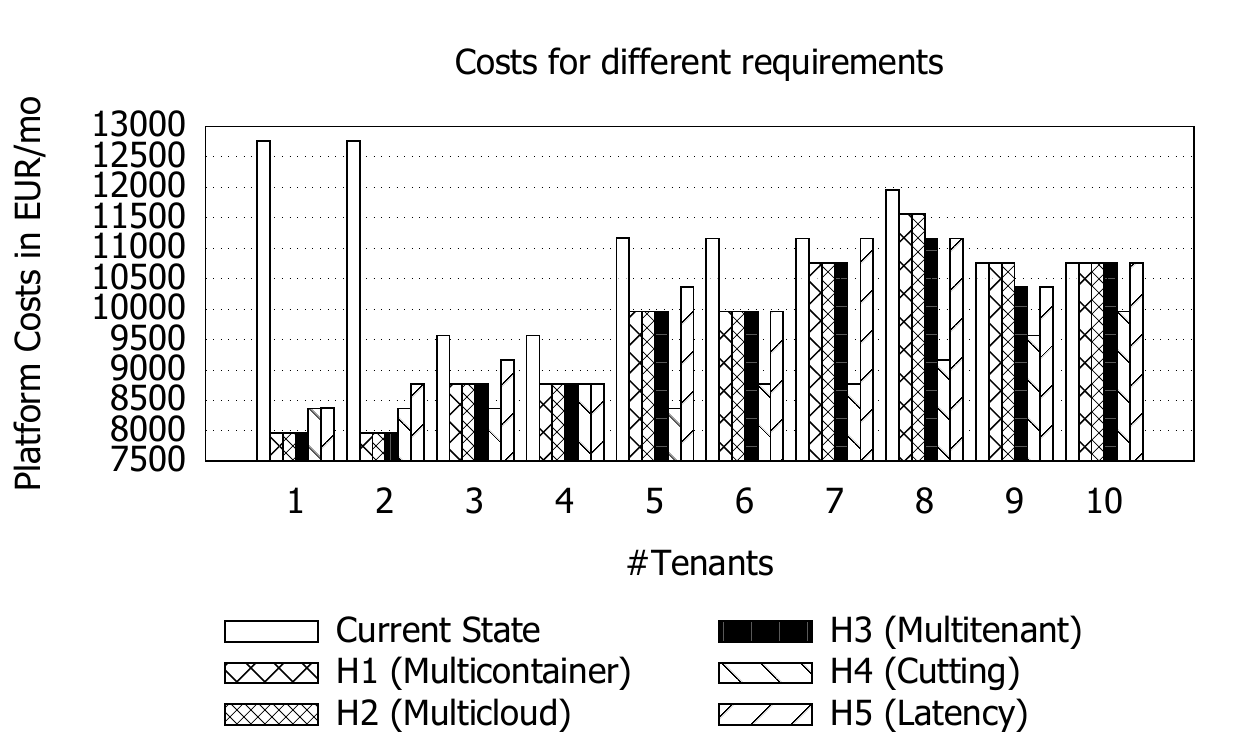}
	%%\vspace{-.7cm}
	\caption{Hypotheses in comparions}
	\label{fig:hypoComparison}
	%%\vspace{-0.3cm}
\end{figure}

\begin{figure}[bt]
	\centering
	\includegraphics[width=1\columnwidth]{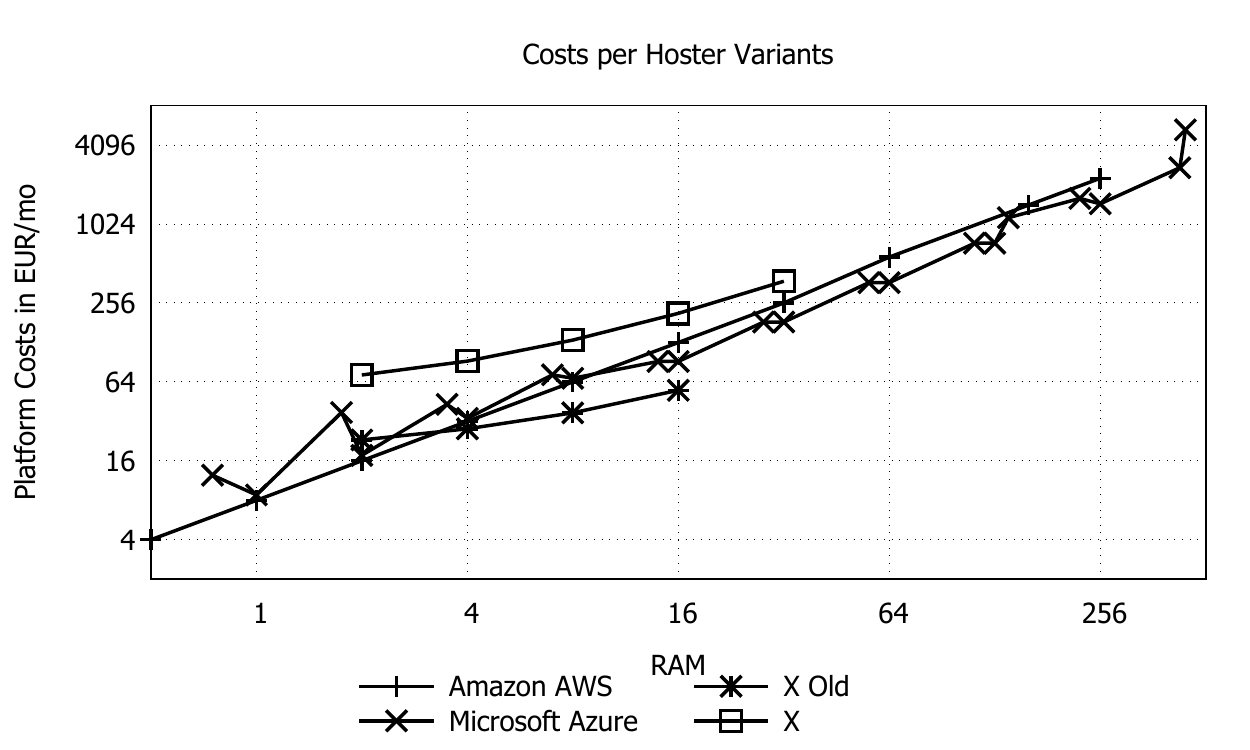}
	%%\vspace{-.7cm}
	\caption{Cost models (H7)}
	\label{fig:costModels}
	%%\vspace{-0.3cm}
\end{figure}

% - compare current approach: all compositions of one tenant in one VM or container using generated heatmaps?? with other approaches\\

\labeltitle{SAP Cloud Platform Integration: eDocuments} The eDocument Electronic Invoicing is a solution for country-specific document management \cite{sap-hci-content}, allowing firms to interact with legal authorities. % (\eg implement the new \emph{EU Data Protection Regulation}\footnote{EU --- General Data Protection Regulation: \url{http://goo.gl/Ru0slz}.}).

\labelsubtitle{Setup} The dataset for country solutions like Italy and Spain contains $13$ distinct compositions (six with non-shareable sub-compositions), which we study for a uniform distribution over an increasing number of virtual tenants (due to confidentiality regulations).
% with three tenants, all compositions: 13, reduction of approximately 18\% /mo w.r.t. no cutting solutions and probably the normal solution due to three containers for three tenants and no mixing.

\labelsubtitle{Results} The costs and savings for the calculated partitions compared to a hosting solution are shown in~\cref{fig:costs_savings} as \texttt{cloud}.
Notably, \enquote{cutting} non-shareable sub-compositions into $19$ distinct compositions is not beneficial in the one-tenant case, however, preferable for more tenants (cf. cost-savings).
Working with the original compositions becomes profitable from five tenants onwards.
The solver latencies for original and cut compositions vary between 500ms and 2.7s, respectively.
The solution for the 19 \enquote{cut} compositions and three tenants costs 112.32 EUR/mo (cf.~\cref{fig:cloud_pre-partitioned}) for a separation to three vendor platform variants and identifies free capacity.

\labelsubtitle{Conclusions} (3) \enquote{cutting} is beneficial (cf. H2); (4) small problem sizes are still practically applicable.
% () Less cost reductions compared to hybrid integration processes; () further trade-off between minimal costs and communication latency (between data centers).

\begin{figure}[bt]
	\centering
	\includegraphics[width=1\columnwidth]{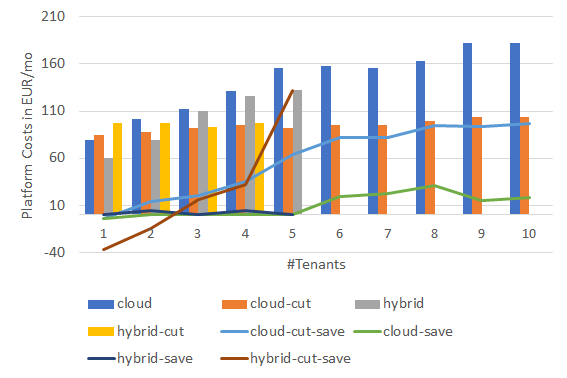}
	%%\vspace{-.7cm}
	\caption{Costs and savings: original and cut} %  37 eDocument (cloud) and 13 C4C-CRM (hybrid) compositions for tenants
	\label{fig:costs_savings}
	%%\vspace{-0.3cm}
\end{figure}

\labeltitle{SAP Cloud Platform Integration: C4C-CRM} The C4C solutions for the communication with on-premise Customer Relationship Management (CRM) applications~\cite{sap-hci-content}, %Enterprise Resource Planning (ERP) and \emph{c4c-erp} and
abbreviated \emph{c4c-crm}~\cite{sap-hci-content}, can be considered a typical hybrid, corporate to cloud application integration~\cite{Ritter201736}.
The dominant integration styles --- according to the classification in~\cite{Ritter201736} --- are process invocation and data movement.
The state changes (\eg create, update) of business objects (\eg business partner, opportunity, activity) as well as master data in the cloud or corporate applications (\eg CRM, ERP) are exchanged with each other.

\labelsubtitle{Setup} The dataset features 37 distinct compositions (seven with non-shareable sub-compositions), which we uniformly distributed over an increasing number of virtual tenants as \texttt{hybrid}.
For the non-cut compositions, platform vendor \enquote{stickiness} is enabled.

\labelsubtitle{Results} The cost-savings for $78$ \enquote{cut} compositions, depicted in~\cref{fig:costs_savings}, make configurations with more than two tenants and five tenants compared to c4c-crm more profitable.
This can be explained due the higher number of compositions, however, with a better shareablity ratio.
On the downside the solver times reach up to 2h for the latter, which makes it not applicable in praxis (\ie no entries beyond five tenants).
The optimal solution for the 37 original compositions and three tenants is shown in~\cref{fig:c4c_normal_partitioning}.
The selected six platform variants from two vendors cost 109.85 EUR/mo.
Due to stickiness constraints (all compositions on one platform) for the non-cut compositions, this solution is close to a hosting approach.
While the transmission latencies of these compositions remain low, there are only minor cost-savings.
Without \enquote{sticky} platform assignments and cut compositions, the cost-savings are high, however, with higher latencies due to the additional remote call (cf.~\cref{fig:nonshareable_rewriting}).

%The optimization took xh to calculate an optimal partitioning for a k-partitioning with the original pattern compositions (\texttt{normal}) shown in~\cref{fig:c4c_normal_partitioning} and zh with an additional pre-partitioning according to non-shareable sub-compositions (cf.~\cref{alg:cutting}), resulting to y partitions as shown in~\cref{fig:c4c_pre-partitioned}.
%With a estimated hosting costs of r EUR/mo, the cost reduction...

\labelsubtitle{Conclusions} (5) on-line heuristics required; (6) trade-off between latency and cost-savings.
% significant cost-savings compared to the eDocuments (higher amount of shareable compositions); 

\begin{figure*}[tb]
	\begin{center}$
		\begin{array}{cc}
		% runtime: 
		\subfigure[eDocuments, pre-partitioned / cut (costs=112.32 EUR/mo)]{\label{fig:cloud_pre-partitioned}\includegraphics[width=0.5\linewidth]{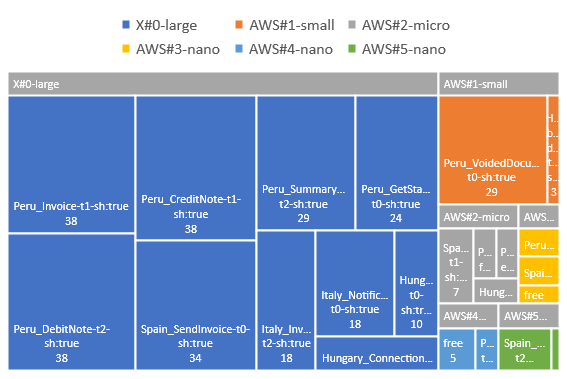}} &
		% runtime: 3,601,980 ms
		\subfigure[C4C-CRM, normal (costs=109.85 EUR/mo)]{\label{fig:c4c_normal_partitioning}\includegraphics[width=0.5\linewidth]{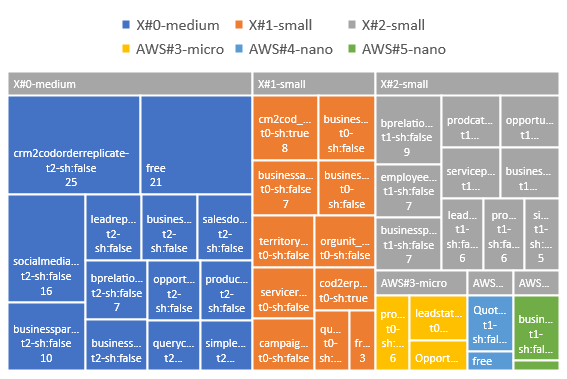}}
		\end{array}$
	\end{center}
	%%\vspace{-.5cm}
	\caption{SAP CPI eDocuments and C4C-CRM compositions from 2016, $tx$ tenants with $x \in\{0,1,2\}$ (anonymized)} %, \small with reference platform as X, Amazon Web Services as AWS, and Microsoft Azure (not selected); Format: \emph{platform}-\emph{costs/mo}-\emph{\#CPUs-RAM(GB)}}
	\label{fig:}
\end{figure*}

%\begin{figure*}[tb]
%	\begin{center}$
%		\begin{array}{cc}
%		% runtime: 3,601,980 ms
%		\subfigure[Normal (costs=11,232 EUR/mo), similar to hosting]{\label{fig:cloud_normal_partitioning}\includegraphics[width=0.5\linewidth]{images/sap_cloud_three_tenants_no_cutting_sorting_binpacking_per_composition}} &
%		% runtime: 
%		\subfigure[Pre-Partitioned (costs=8,410 EUR/mo)]{\label{fig:cloud_pre-partitioned}\includegraphics[width=0.5\linewidth]{images/sap_cloud_three_tenants_with_cutting_sorting_binpacking_per_composition}}
%		\end{array}$
%	\end{center}
%	%%%\vspace{-.5cm}
%	\caption{$13$ SAP eDocuments compositions from 2016 for three tenants (anonymized), \small with reference platform as X, Amazon Web Services as AWS, and Microsoft Azure (not selected); Format: \emph{platform}-\emph{costs/mo}-\emph{\#CPUs-RAM(GB)}}f
%	\label{fig:}
%\end{figure*}

\subsection{Performance}

\subsubsection{Data reduction}
\begin{figure}
  \centering
  \includegraphics[width=0.9\columnwidth]{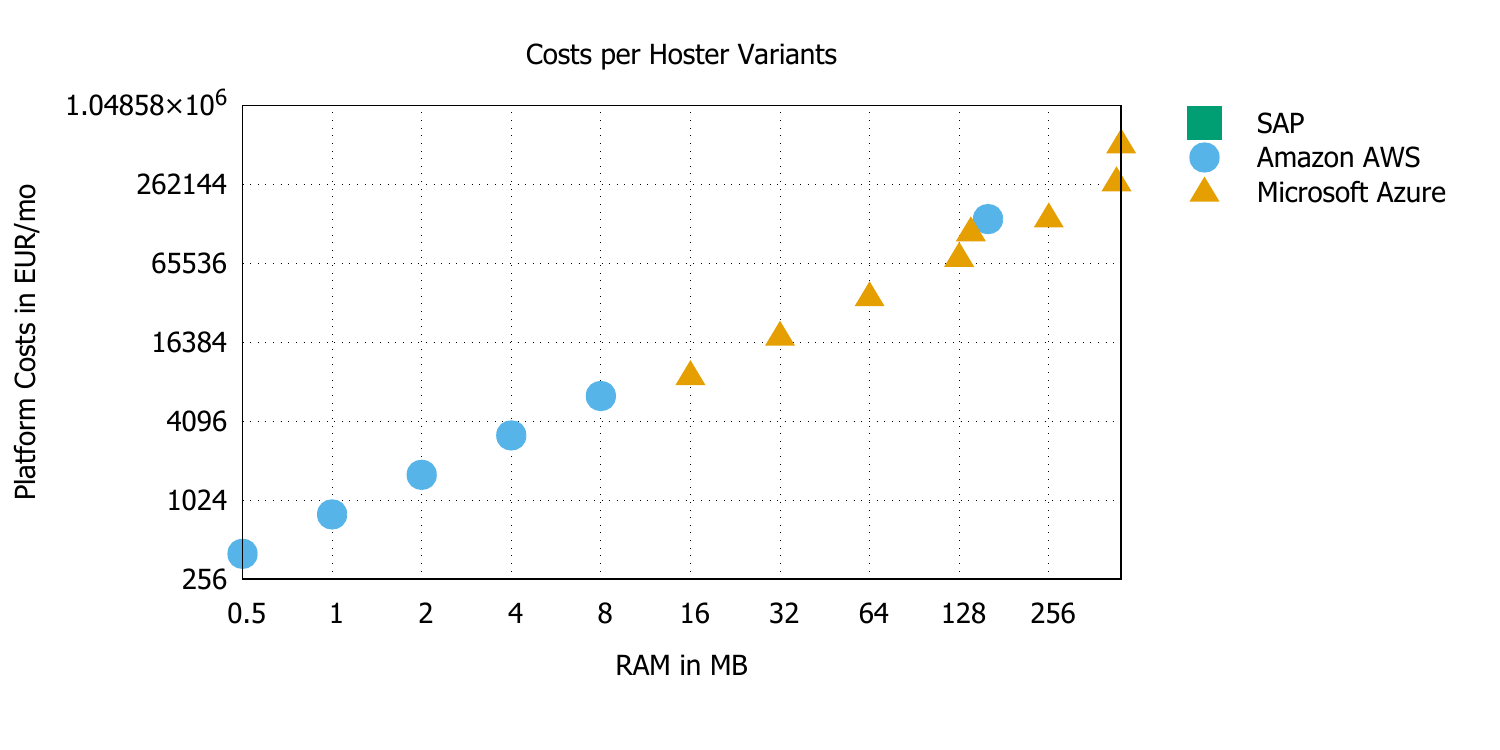} 
  \caption{After removing overly expensive variants (111 $\rightarrow$ 14)}
  \label{fig:variantsWithoutOverlyExpensive}
\end{figure}

\begin{table}[tb]
	\centering
\begin{tabu}{|c|c|>{\centering\arraybackslash}p{3.5cm}|>{\centering\arraybackslash}p{3.5cm}|}
\hline 
 & \multirow{2}{*}{\thead{Number of\\IFlows}} & \multicolumn{2}{c|}{\thead{Percentage Reduction per Bundle Size}} \\ 
\cline{3-4} 
 &  & \thead{64 MB} & \thead{128 MB} \\ 
\tabucline[1.75pt]{-}
\multirow{3}{*}{cloud}         & \multirow{3}{*}{14}           & 42.86\% & 78.57\%\\ 
 &  & 42.86\% & 64.29\%\\
 &  & 28.57\% & 35.71\%\\
\hline 
\multirow{3}{*}{crm}         & \multirow{3}{*}{37}            & 69.77\% & 93.02\%\\ 
 &  & 88.37\% & 88.37\%\\
 &  & 83.72\% & 83.72\%\\
\hline 
\multirow{3}{*}{erp}         & \multirow{3}{*}{43}            & 78.38\% & 91.89\%\\ 
 &  & 86.49\% & 86.49\% \\
 &  & 81.08\% & 81.08\%\\
\tabucline[1.75pt]{-}
\multirow{11}{*}{\makecell{generated\\data}} & 50 & 72.00\% & 78.00\%\\ 
\cline{2-4} 
 & 100 & 60.00\% & 73.00\%\\ 
\cline{2-4} 
 & 200 &  74.00\% & 82.50\%\\ 
\cline{2-4}  
 & 500 & 74.60\% & 84.20\%\\ 
\cline{2-4}  
 & 1,000 &  77.50\% & 85.00\%\\ 
\cline{2-4}  
 & 2,000 &  74.85\% & 85.50\%\\ 
\cline{2-4}  
 & 5,000 & 76.96\% & 84.58\%\\ 
\cline{2-4}  
 & 10,000 & 74.54\% & 84.02\%\\ 
\cline{2-4}  
 & 50,000 & 75.82\% & 84.02\%\\ 
\cline{2-4}  
 & 100,000 & 75.60\% & 84.26\%\\ 
\cline{2-4}  
 & 170,000 & 75.46\% & 83.98\%\\ 
\hline 
\end{tabu} 
	\caption{Data Reduction due to aggregation of IPCGs to bundles}
	\label{tab:flowBundles}
\end{table}

reduction of model size milp

\begin{table}[!htb]
	\centering
\begin{adjustbox}{max width=\textwidth}
\begin{tabu}{|c|c|r r r|r r r|}
\hline 
& \multirow{2}{*}{\thead{Number of\\IFlows}} & \multicolumn{3}{|c|}{\thead{Variables}} & \multicolumn{3}{|c|}{\thead{Constraints}} \\ 
\cline{3-8} 
 &   & \thead{Original} &  \thead{Adapted} & \thead{Reduction} &  \thead{Original} &  \thead{Adapted} & \thead{Reduction} \\ 
\tabucline[1.75pt]{-}
\multirow{3}{*}{cloud}         & \multirow{3}{*}{14}            &2,289     & 903     & 60.55\%   & 3,673        & 440     & 88.02\%   \\
 &  & 2,616     & 1,032    & 60.55\%   & 4,196        & 581     & 86.15\%   \\
 &  & 2,616     & 1,032    & 60.55\%   & 4,196        & 637     & 84.82\%   \\
\hline 
\multirow{3}{*}{crm}         & \multirow{3}{*}{37}            & 9,138     & 912     & 90.02\%   & 23,243       & 2,730    & 88.25\%   \\
 &  & 9,138     & 912     & 90.02\%   & 23,243       & 3,246    & 86.03\%   \\
 &  & 12,184    & 1,216    & 90.02\%   & 30,979       & 4,644    & 85.01\%   \\
\hline 
\multirow{3}{*}{erp}         & \multirow{3}{*}{43}             & 14,063    & 1,106    & 92.14\%   & 35,727       & 4,123    & 88.46\%   \\
 &  & 12,054    & 948     & 92.14\%   & 30,629       & 4,242    & 86.15\%   \\
 &  & 16,072    & 1,264    & 92.14\%   & 40,825       & 6,058    & 85.16\%   \\
\tabucline[1.75pt]{-}
\multirow{6}{*}{\makecell{generated\\data}} & 5  & 294      & 240     & 18.37\%   & 163         & 28      & 82.82\%   \\
\cline{2-8} 
 & 10 & 681      & 375     & 44.93\%   & 920         & 30      & 96.74\%   \\
\cline{2-8} 
 & 20 & 5,370     & 1,350    & 74.86\%   & 11,768       & 919     & 92.19\%   \\
\cline{2-8} 
 & 50 & 18,669    & 1,155    & 93.81\%   & 48,866       & 5,908    & 87.91\%   \\
\cline{2-8} 
 & 100 & 275,859   & 5,805    & 97.90\%   & 770,354      & 112,095  & 85.45\% \\
\cline{2-8} 
 & 200 & 1,048,242  & 8,190    & 99.22\%   & 2,975,664     & 447,997  & 84.94\% \\
\hline 
\end{tabu}
\end{adjustbox}
	\caption{Reduction of model size for the adapted MILP-model}
	\label{tab:modelSizeComparison}
\end{table}

performance

\begin{table}[!htb]
	\centering
\begin{adjustbox}{max width=\textwidth}
\begin{tabu}{|c|c|r|r|c|}
\hline
 & \thead{Number of\\IFlows} & \thead{Original\\Model} & \thead{Adapted\\Model} & \thead{Percentage\\Improvement}      \\
\tabucline[1.75pt]{-}
\multirow{3}{*}{cloud}         & \multirow{3}{*}{14}                     & 1,009.25     & 213.13   & 78.88\% \\
               &               & 1,360.89     & 661.25   & 51.41\% \\
               &               & 2,800.84     & 699.28   & 75.03\% \\
\hline
\multirow{3}{*}{crm}         & \multirow{3}{*}{37}                       & 140,280.99   & 2,864.62  & \color[HTML]{228B22}97.96\% \\
               &               & 5,764.71     & 1,114.58  & 80.67\% \\
               &               & 13,883.36    & 2,599.72  & 81.27\% \\
\hline
\multirow{3}{*}{erp}         & \multirow{3}{*}{43}                      & 488,715.37   & 6,017.97  & \color[HTML]{228B22}98.77\% \\
               &               & 22,944.36    & 1,316.69  & \color[HTML]{228B22}94.26\% \\
               &               & 157,141.00   & 4,826.37  & \color[HTML]{228B22}96.93\% \\
\tabucline[1.75pt]{-}
generated Data & 5             & 22.50       & 9.82     & 56.33\% \\
\cline{3-5}
               & 10            & 116.88      & 32.83    & 71.91\% \\
\cline{3-5}
               & 20            & 52,040.20    & 3,034.24  & \color[HTML]{228B22}94.17\% \\
\cline{3-5}
               & 50            & 600,604.67   & 31,770.72 & \color[HTML]{228B22}94.71\% \\
\hline
\end{tabu}
\end{adjustbox}
	\caption{Comparison of computation time between original and adapted MILP-model}
	\label{tab:milpPerformanceOriginalVsAdapted}
\end{table}

\begin{table}[!htb]
	\centering
\begin{adjustbox}{max width=\textwidth}
\begin{tabu}{|c|c|r|r|r|r|r|}
\hline
 & \multirow{2}{*}{\thead{Number of\\IFlows}} & \multirow{2}{*}{\thead{Raw Adapted\\Model}} & \multicolumn{3}{|c|}{\thead{Improvement for Data Reduction}}     & \multirow{2}{*}{\thead{Improvement for\\Decomposition}} \\
 \cline{4-6}
 &&&\thead{Variants} & \thead{IFlows} & \thead{Variants + IFlows}     &  \\
\tabucline[1.75pt]{-}
\multirow{3}{*}{cloud}         & \multirow{3}{*}{14}                         & 213.13   & 24.32\%                          & 46.71\%                        & 42.29\%                        & {\color[HTML]{FE0000} -3378.04\%}  \\
               &                   & 661.25   & 24.97\%                          & 76.44\%                        & 76.61\%                        & {\color[HTML]{FE0000} -1942.38\%}  \\
               &                   & 699.28   & 20.26\%                          & 44.12\%                        & 43.01\%                        & {\color[HTML]{FE0000} -1782.00\%}  \\
\hline
\multirow{3}{*}{crm}         & \multirow{3}{*}{37}                         & 2,864.62  & {\color[HTML]{FE0000} -13.79\%}  & {\color[HTML]{228B22} 95.79\%} & {\color[HTML]{228B22} 95.83\%} & {\color[HTML]{FE0000} -158.82\%}   \\
               &                   & 1,114.58  & {\color[HTML]{FE0000} -14.89\%}  & {\color[HTML]{228B22} 97.82\%} & {\color[HTML]{228B22} 97.83\%} & {\color[HTML]{FE0000} -1134.81\%}  \\
               &                   & 2,599.72  & 3.45\%                           & {\color[HTML]{228B22} 98.56\%} & {\color[HTML]{228B22} 98.74\%} & {\color[HTML]{FE0000} -604.82\%}   \\
\hline
\multirow{3}{*}{erp}         & \multirow{3}{*}{43}                      & 6,017.97  & 20.45\%                          & {\color[HTML]{228B22} 94.06\%} & {\color[HTML]{228B22} 96.19\%} & {\color[HTML]{FE0000} -8.88\%}     \\
               &                   & 1,316.69  & {\color[HTML]{FE0000} -52.63\%}  & {\color[HTML]{228B22} 98.19\%} & {\color[HTML]{228B22} 98.52\%} & {\color[HTML]{FE0000} -854.67\%}   \\
               &                   & 4,826.37  & 3.29\%                           & {\color[HTML]{228B22} 99.16\%} & {\color[HTML]{228B22} 99.11\%} & {\color[HTML]{FE0000} -272.39\%}   \\
\tabucline[1.75pt]{-}
\multirow{4}{*}{\makecell{generated\\data}} & 5                 & 9.82     & 72.11\%                          & {\color[HTML]{FE0000} -9.45\%} & 74.26\%                        & {\color[HTML]{FE0000} -56420.41\%} \\
\cline{2-7}
               & 10                & 32.83    & {\color[HTML]{FE0000} -274.34\%} & 59.57\%                        & 65.52\%                        & {\color[HTML]{FE0000} -9637.04\%}  \\
\cline{2-7}
               & 20                & 3,034.24  & {\color[HTML]{FE0000} -5.70\%}   & {\color[HTML]{228B22} 92.31\%} & {\color[HTML]{228B22} 93.55\%} & {\color[HTML]{FE0000} -354.04\%}   \\
\cline{2-7}
               & 50                & 31,770.72 & {\color[HTML]{FE0000} -38.88\%}  & {\color[HTML]{228B22} 99.19\%} & {\color[HTML]{228B22} 98.90\%} & 41.51\%     \\                       
\hline
\end{tabu}
\end{adjustbox}
	\caption{Changes in computation time for data reduction and decomposition}
	\label{tab:milpPerformanceStrategies}
\end{table}

solution quality

\begin{table}[!htb]
	\centering
\begin{adjustbox}{max width=\textwidth}
\begin{tabu}{|c|c|r|r r|r r|}
\hline
   & \multirow{2}{*}{\thead{Number of\\IFlows}} & \multicolumn{1}{|c|}{\multirow{2}{*}{\thead{Optimal\\Result}}} & \multicolumn{2}{|c|}{\thead{Bundled IFlows}}     & \multicolumn{2}{|c|}{\thead{Decomposition}}           \\
\cline{4-7}
   & &   & \thead{Result} & \thead{Deviation} & \thead{Result} & \thead{Deviation} \\
\tabucline[1.75pt]{-}
\multirow{3}{*}{cloud}         & \multirow{3}{*}{14}             & 2,388    & 2,388   & \textbf{0.00\%}    & 2,786          & 16.67\%   \\
               &     & 2,786    & 2,786   & \textbf{0.00\%}    & 3,184          & 14.29\%   \\
               &     & 3,184    & 3,184   & \textbf{0.00\%}    & 3,184          & \textbf{0.00\%}     \\
\hline
\multirow{3}{*}{crm}         & \multirow{3}{*}{37}             & 2,388    & 2,388   & \textbf{0.00\%}     & 2,388          & \textbf{0.00\%}     \\
               &     & 1,990    & 1,990   & \textbf{0.00\%}     & 2,388          & 20.00\%   \\
               &     & 2,786    & 2,786   & \textbf{0.00\%}     & 3,184          & 14.29\%   \\
\hline
\multirow{3}{*}{erp}         & \multirow{3}{*}{43}              & 2,388    & 2,388   & \textbf{0.00\%}     & 2,786          & 16.67\%   \\
               &     & 1,990    & 1,990   & \textbf{0.00\%}     & 2,388          & 20.00\%   \\
               &     & 2,786    & 2,786   & \textbf{0.00\%}     & 3,184          & 14.29\%   \\
\tabucline[1.75pt]{-}
\multirow{6}{*}{\makecell{generated\\data}}  & 5   & 796     & 796    & \textbf{0.00\%}     & 1,194          & 50.00\%   \\
\cline{2-7}
               & 10  & 1,194    & 1,195   & 8.38\%    & 1,592          & 33.33\%   \\
\cline{2-7}
               & 20  & 3,582    & 3,584   & 5.58\%    & 3,980          & 11.11\%   \\
\cline{2-7}
               & 50  & 3,983    & 3,983   & \textbf{0.00\%}     & 4,379          & 9.94\%    \\
\cline{2-7}
               & 100 & [$\leq$ 14,734]      & 14,336  & -         & 14,333         & -         \\
\cline{2-7}
               & 200 & [$\leq$ 2,088,150]       & 25,102  & -         & 25,488         & -     	\\  
\hline
\end{tabu}
\end{adjustbox}
	\caption{Comparison of result quality for approximated results using a MILP-solver}
	\label{tab:milpResultQuality}
\end{table}

local search - 

\subsection{Discussion} \todo[inline]{add decision support or rule of thumb on when it is beneficial} The experiments motivate design decision of our CEPP solution realization, as well study the problem itself.
Although the problem is inherently intractable from a complexity perspective (cf. conclusion (5)), which requires on-line heuristics probably leading to more expensive solutions, the optimal solution that we propose could be used to find cheaper solutions for real-world datasets from SAP CPI (conclusions (1)+(2)+(4)).
This resulted in first insights into different aspects of the problem like trade-offs of more cost optimal results for cut-compositions (cf. conclusion (3)) and the connected preference for compositions with a higher shareability ratio ($\rightarrow$ revisit how content is developed), as well as latency and cost-savings (cf. conclusion (6)).
% () further trade-off between minimal costs and communication latency (between data centers).
We observe that non of the Microsoft Azure containers was selected, potentially due to a special cost structure, which has to be studied further.

\section{Cost-efficient placement model (old)} \label{sec:milp_old}

In this section, we define an optimization model for the CEPP, which we base on the multicloud INTaaS model.
For the sake of clarity,~\cref{tab:model} summarizes the notation used throughout this work.

\begin{table}[tb]
	\centering
	\begin{tabular}{|c|c|c|}
		\hline
		Control Variable & Used to Iteration over & Upper Bound\\
		\hline
		$i$ & integration flows & F\\
		\hline
		$j$ & containers & C\\
		\hline
		$n$ & variants & V\\
		\hline
	\end{tabular}
	\caption{Control variables used in MILP-model definition}
	\label{tab:milpControlVariables}
\end{table}

\begin{table}[tb]
	\scriptsize
	\centering
	\caption{Overview of used variables in the cost model}
	\label{tab:model}
	%\vspace{-0.3cm}
	\begin{tabular}{|l|l|}
		\hline
		Symbol & Description \\ \hline
		$F$ & The number of compositions \\
		$C$ & The number of containers provided for solving \\
		$x_{ij}$ & Boolean indicating if composition i is in container j \\
		$A_i$ & Required capacity for composition i \\
		$B_j$ & Capacity of container j \\
		$G_j$ & Costs of container j \\
		$\beta_{ij}$ & Capacity of composition i for container j (0 if $x_{ij} = 0$, $A_i$ if $x_{ij} = 1$) \\
		$W$ & $\max A_i$ \\
		$V$ & $\max E_n $ \\
		$S$ & $\max \mu_n$ \\
		$Q$ & Maximum number of compositions in one container \\
		$T_i$ & Tenant of composition i \\
		$z_{ikj}$ & Composition k with side effects is in same container j as composition i \\
		$y_{nj}$ & Container j is variant n \\
		$D_n$ & Capacity of variant n \\
		$E_n$ & Costs of variant n \\
		$H_j$ & Number of compositions in container j \\
		$P_j$ & Boolean indicating if container j contains at least 1 composition \\
		$\alpha_j$ & Costs of container j if used (0 if $P_{j} = 0$, $G_j$ if $P_{j} = 1$) \\
		$\mu_n$ & Provider of variant n \\
		$\omega_j$ & Provider of container j \\
		$U_{ij}$ & Provider of composition i in container j (0 if $x_{ij} = 0$, $\omega_j$ if $x_{ij} = 1$)\\
		$R_i$ & Provider of composition i \\
		$\gamma_{ip}$ &  Boolean indicating if provider k is provider of composition  (1 if $p = R_i$, else 0)\\
		$p_{t}$ &  Number of preferred providers of tenant $t$\\
		$p_{tk}$ &  Provider no.$k$ (with $1 \leq k \leq p_t$) which is preferred by tenant $t$\\
		$l$ & Latency per cut, if compositions are not on same container\\
		$L$ & Maximum additional latency per composition
		\\ \hline
	\end{tabular}
	%\vspace{-.3cm}
\end{table}

\begin{table*}[tb]
	\centering
	\begin{adjustbox}{max width=\textwidth}
	\begin{tabular}{|c|c|l|c|}
		\hline
		&\textbf{Variable} & \textbf{Meaning} & \thead{In Adapted \\ Model}  \\ 
		\hline
		\parbox[t]{2mm}{\multirow{4}{*}{\rotatebox[origin=c]{90}{\small Constants}}} 
		&$D_n$ & Capacity of variant $n$  & x\Tstrut\\
		&$E_n$ & Costs of variant $n$ & x \\
		&$A_i$ & Required capacity for flow $i$ & x \\
		&$Q$ & Maximum number of flows per container & x\Bstrut\\
		\hline
		\parbox[t]{2mm}{\multirow{2}{*}{\rotatebox[origin=c]{90}{\small Result}}} &$x_{ij}$ & Boolean indicating if composition $i$ is in container $j$& x\Tstrut\\
		&$y_{nj}$ & Container j is variant n   & x\Bstrut\\
		\hline
		\parbox[t]{2mm}{\multirow{7}{*}{\rotatebox[origin=c]{90}{\small Auxiliary Variables}}}&$B_j$ & Capacity of container j & x\Tstrut\\
		&$G_j$ & Costs of container j & x \\
		&$\beta_{ij}$ & Capacity of flow $i$ for container $j$ (0 if $x_{ij} = 0$, $A_i$ if $x_{ij} = 1$)  & \\
		&$z_{ikj}$ & Flow $k$ is in same container j as flow $i$ & x  \\
		&$H_j$ & Number of flows in container $j$  &   \\
		&$P_j$ & Boolean indicating if container $j$ contains at least one flow  & \\
		&$\alpha_j$ & Costs of container $j$ if used (0 if $P_{j} = 0$, $G_j$ if $P_{j} = 1$) & \Bstrut\\
		\hline
	\end{tabular}
	\end{adjustbox}
	\caption{Overview of used variables in the cost model}
	\label{tab:milpVariables}
\end{table*}

\begin{table*}[tb]
\centering
\begin{tabular}{|c|c|c|}
\hline 
 & \thead{Original Model} & \thead{Adapted Model} \\ 
\hline 
\makecell{\ref{item:flowConstraint}\\Flow in exactly\\ one container} & \multicolumn{2}{|c|}{{$\!\begin{aligned}
	\sum_{j=1}^{C}x_{ij} = 1 & & \forall i
	\end{aligned}$}} \\ 
\hline 
\makecell{\ref{item:containerConstraint}\\Container is exactly\\ one variant} & \multicolumn{2}{|c|}{{$\!\begin{aligned}
	\sum_{n=1}^{N}y_{nj} = 1 & & \forall j 
	\end{aligned}$}} \\ 
\hline 
\makecell{\ref{item:sizeConstraint}\\Container size\\not exceeded} & {$\!\begin{aligned}
	&&\sum_{i=1}^{F}\beta_{ij} &\leq B_j && \forall j && \\
	\text{With:} && A_i &\leq W\cdot (1-x_{ij}) + \beta_{ij} && \forall i,j  \\
	&&\beta_{ij} &\leq A_i && \forall i,j  \\
	&&\beta_{ij} &\leq W \cdot x_{ij} && \forall i,j \\
	&&\beta_{ij} &\geq 0 && \forall i,j
	\end{aligned}$} & {$\!\begin{aligned}\sum_{i=1}^{F}A_i \cdot x_{ij} \leq B_j & & \forall j\end{aligned}$} \\ 
\hline 
\makecell{\ref{item:securityConstraint}\\Security\\awareness} & {$\!\begin{aligned}
	&& T_i \cdot z_{ikj} &= T_k \cdot z_{ikj} && \forall j && \\[12pt]
	\text{With:} && x_{ij} + x_{kj} - 1 &\leq z_{ikj} && \forall i,j,k  \\
	&&z_{ikj} &\leq x_{ij} && \forall i,j,k  \\
	&&z_{ikj} &\leq x_{kj} && \forall i,j,k  
	\end{aligned}$} & {$\!\begin{aligned}x_{ij} + x_{kj} \leq 1 & & \forall j\end{aligned}$} \\ 
\hline 
\makecell{\ref{item:maxFlowNumber}\\Max. flow number\\not exceeded} & \multicolumn{2}{|c|}{{$\!\begin{aligned}
	&& H_j &\leq Q && \forall j && \\
	\text{With:} && H_j &= \sum_{i=1}^{F}x_{ij} && \forall j
	\end{aligned}$}} \\ 
\hline 
\makecell{\textbf{Objective}} & 	{$\!\begin{aligned} 
	&& \min &\sum_{j=1}^{C}\alpha_j && && \\
	\text{With:} && P_j &\leq H_j && \forall j\\
	&& H_j &\leq Q \cdot P_j && \forall j  \\
	&& G_j &\leq V \cdot (1-P_j) + \alpha_j && \forall j \\
	&&\alpha_j &\leq G_j && \forall j \\
	&& \alpha_j &\leq V \cdot P_j && \forall j 
	\end{aligned}$} & $\min \sum_{j=1}^{C} G_j$ \\ 
\hline 
\end{tabular} 
\caption{Comparison of the original and adapted MILP-model}
\label{tab:modelComparison}

\end{table*}

% todo: where to add the variants: cutting, bin-packing as pre-processing? maybe in the realization section?\\

% \subsection{Security Constraint Model}
\labeltitle{Basic Constraints} We first consider basic constraints like every composition i must be in exactly one container j at a time,
% We have chosen to use a mixed integer linear programming approach (MIP) to model our cost function, as there exist open source and commercial solvers like GLPK \cite{glpk} designed for solving these problems. Furthermore, it is possible to create and use existing heuristics like pivot and shift \cite{balas2004pivot} for solving optimization problems modelled as MIP.
% - Every composition can physically only be in one container at a time.
\begin{align*}
x_{ij} \in \{0,1\} \\
\sum_{j=1}^{C}x_{ij} = 1 &&\forall i
\end{align*}
with Boolean $x_{ij}$ indicating if composition i is in container j and the maximal number of containers $C$ in the solution.
Thereby, the used capacity of container j is calculated by the maximal required composition capacities $A_i$, with an auxiliary symbol $\beta_{ij}$ for the required capacity of composition $i$ on container $j$,
\begin{align*}
W &= \max A_i \\
A_i &\leq W\cdot (1-x_{ij}) + \beta_{ij} &&\forall i,j \\
\beta_{ij} &\leq A_i &&\forall i,j \\
\beta_{ij} &\leq W \cdot x_{ij} &&\forall i,j \\
\beta_{ij} &\geq 0 &&\forall i,j
\end{align*}
and the constraint that the combined required composition capacities in container j must be lower than or equal to the capacity of the container itself $B_j$ for all compositions $F$.
\begin{align*}
\sum_{i=1}^{F}\beta_{ij} \leq B_j &&\forall j
\end{align*}

\labeltitle{Security-aware} According to the shareability requirement $z_{ikj}$, no composition $k$ with potential side-effects can be in the same container j as another tenants composition i.
Thereby, $T_i$ and $T_k$ denote the tenant of the compositions $i,k$.
\begin{align*}
x_{ij} + x_{kj} - 1 &\leq z_{ikj} &&\forall i,j,k \\
z_{ikj} &\leq x_{ij} &&\forall i,j,k \\
z_{ikj} &\leq x_{kj} &&\forall i,j,k \\
T_i \cdot z_{ikj} &= T_k \cdot z_{ikj} &&\forall i,j,k
\end{align*}

\labeltitle{Containers and variants} We need to determine which container variants $n$ are used by the containers $y_{nj}$ and make sure that every container $j$ is assigned with exactly one variant,  
\begin{align*}
y_{nj} \in \{0,1\} \\
\sum_{n=1}^{N}y_{nj} = 1 &&\forall j
\end{align*}
while ensuring that according to the chosen variant with capacity $D_n$ of the container $j$ and the variant's costs $E_n$, the container's capacity $B_j$ and costs $G_j$ are set correctly.
\begin{align*}
B_j &= \sum_{n=1}^{N} D_n \cdot y_{nj} &&\forall j \\
G_j &= \sum_{n=1}^{N} E_n \cdot y_{nj} &&\forall j	
\end{align*}

\labeltitle{Container costs} Let $H_j$ be the auxiliary variable denoting the number of compositions that are on container $j$ and assign its value, with the maximum number of compositions in one container $Q$.
\begin{align*}
H_j &= \sum_{i=1}^{F}x_{ij} &&\forall j\\
H_j &\leq Q &&\forall j
\end{align*}
As an upper boundary for the number of containers, we use $H_j$ to assign a Boolean value $P_j$ indicating whether container $j$ contains any composition.
% This is needed as we cannot know the amount of containers before and therefore provide a number that is probably to big.
\begin{align*}
P_j &\in \{0,1\} \\
P_j &\leq H_j &&\forall j\\
H_j &\leq Q \cdot P_J &&\forall j
\end{align*}
Now we define the container costs $\alpha_j$, but only if it is used. 
Unused containers are assumed to be not charged (as in current cloud platforms), and thus do not contribute to the overall costs.
\begin{align*}
V &= \max E_n \\
G_j &\leq V \cdot (1-P_j) + \alpha_j &&\forall j\\
\alpha_j &\leq G_j &&\forall j \\
\alpha_j &\leq V \cdot P_j &&\forall j
\end{align*}

\begin{figure*}[tb]
	\centering
	\includegraphics[width=.7\linewidth]{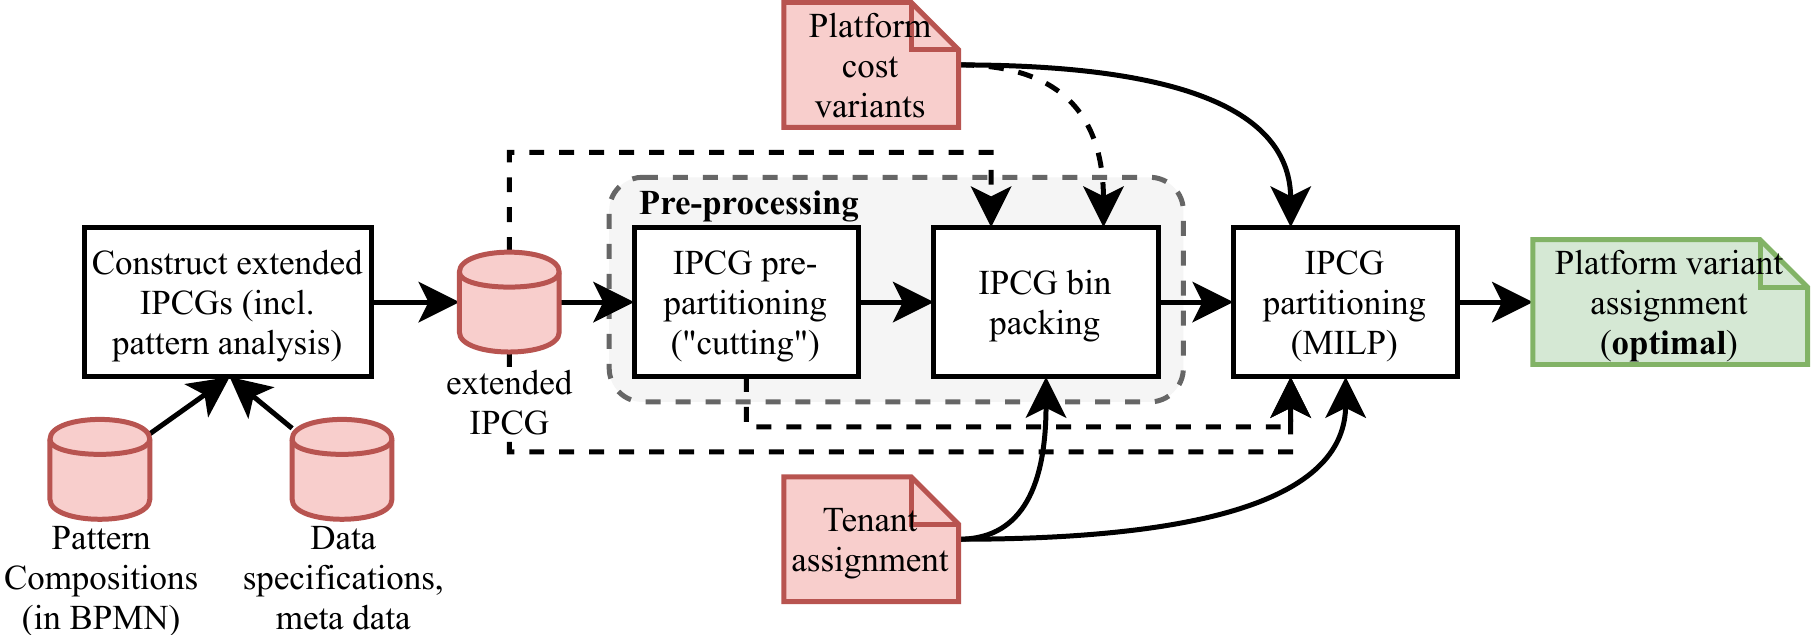}
	% \caption{Realization approach: from BPMN pattern compositions to an optimal platform variant assignment}
	\caption{CEPP solution realization}
	\label{fig:realization_approach}
\end{figure*}

\labeltitle{Stickiness} For reasons like latency reduction or business preferences all compositions of one tenant should be hosted on the same platform, which we model subsequently as optional constraints.
% Furthermore, we additionally thought of a way of modelling that compositions of the same tenant are hosted on the same platform as this may be required for certain tenants to reduce latency. 
% As this increases the complexity of the model we made these constraints optional.
First, let provider $\omega_j$ value determined by its variant through $\mu_n$ provider of variant $n$ and $y_{nj}$ container j is variant n.
\begin{align*}
\omega_j &= \sum_{n=1}^{N} \mu_n \cdot y_{nj} &&\forall j \\
S &= \max \mu_n
\end{align*}
With the auxiliary symbol $U_{ij}$, denoting the provider of composition $i$ in container $j$,
\begin{align*}
\omega_j &\leq S \cdot (1 - x_{ij}) + U_{ij} &&\forall i,j \\
U_{ij} &\leq \omega_j &&\forall i,j \\
U_{ij} &\leq S \cdot x_{ij} &&\forall i,j \\
U_{ij} &\geq 0 &&\forall i,j
\end{align*}
we get the provider of composition i, and add up all the auxiliary variables $U_{ij}$ for all compositions $i$.
\begin{align*}
R_i = \sum_{j=1}^{C}U_{ij} && \forall i
\end{align*}
Finally, to ensure every composition of the tenant $t$ is hosted on the same provider we constraint the composition providers $R_i$.
% model that the provider of every composition $l_m$ of tenant $t$ is the same as the provider of the first composition of this tenant. 
\begin{align} \label{eq:stickiness}
R_{i_1} = {R_i}_m && \text{For all compositions} \ i_m \ \text{of tenant} \ t 
\end{align}

\labeltitle{Latency} To restrict network latencies resulting from partitioned pattern compositions $z_{ikj}$ across different platforms, we introduce an upper threshold $L$, which ensures that for each composition the specified constraint values is not exceeded.
The auxiliary variable $l$ denotes the latency per cut.
\begin{align*}
\sum_{j=1}^C \sum_{k\in K}  (l \cdot x_{ij} - l \cdot z_{ikj}) \leq L && \forall i \\
K \text{ is the set of cuts from flow } i\\
\end{align*}

\labeltitle{Vendor Preferences} To ensure that compositions of a tenant are placed on a container hosted by one of his preferred vendors, the number of preferred hosters $p_t$ for tenant $t$  must be positive. 
\begin{align*}
p_{t} &> 0 && \forall t
\end{align*}
The variable $p_{tk}$ defines the $k$th preferred vendor of tenant $t$, while $\gamma_{ip}$ is a boolean indicating if provider $p$ is provider of composition $i$. If only one vendor is preferred all flows must be placed on its containers.
Otherwise the compositions can be distributed on containers of any preferred vendor. 
\begin{align*}
R_i&=\begin{cases}
p_{{T_i} 1} & p_{T_i} = 1\\
\sum_{k=1}^{p_{T_i}}p_{{T_i}k} \cdot \gamma_{ip_{{T_i}k}} & p_{T_i} >1
\end{cases} && \forall i\\
~~\sum_{k=1}^{p_{T_i}}&\gamma_{ip_{{T_i}k}}=1 ~~~~~~~~~~ (\text{if } p_{T_i} > 1) && \forall i
\end{align*}

% \todo[inline]{vendor preferences, ok?}

\labeltitle{Objective} Now, the minimal costs for the INTaaS vendor are given by the sum of used containers $\alpha_j$:
\begin{align} \label{eq:minimal}
\min \sum_{j=1}^{C}\alpha_j
\end{align}

Note that the proposed model combines INTaaS vendor costs as primary objective, while its customers' compositions processing latencies are sub-constraints that allow the customer to configure latency boundaries.
The customers' preferences with respect to a platform vendor can be taken into account as well.
However, since we target a design time partitioning, dynamic costs like bandwidth are not considered.

\section{Design decisions - Methods}

% Tree Style from https://tex.stackexchange.com/questions/206971/diagram-using-forest-package
%https://tex.stackexchange.com/questions/365338/forest-adjust-tree-edge-path

\begin{figure*}[tb]
	\centering
\begin{forest}
  dir tree switch=at 1,
  for tree={
    font=\sffamily,
    rect,
    align=center,
    edge+={thick, draw=darkgray},
    where level=0{%
      colour me out=black!50!white,
    }{%
      if level=1{%
        colour me out=black!25!white,
      }{%
      	if level=2{%
          colour me out=black!0!white,
          edge+={-Triangle}
        }{%
          edge+={-Triangle},
        }
       },
    },
  }
  [~~~~Problem~~~~
    [\textbf{Model}\\(Formal Problem Representation)
      [Minimize Size / Complexity
      	[Variables]
      	[Constraints]
      ]
      [Decomposition]
    ]
    [\textbf{Data}\\(Real Problem Instance)
      [Reduce Data
      	[Filtering]
      	[Aggregation]
      ]
    ]
    [\textbf{Solving Technique}\\(Result Calculation)
      [Orchestration]
      [Algorithm
  	  	[MILP]
  	  	[Local Search]
  	  ]
    ]
  ]
\end{forest}
	\caption{Potential areas for performance improvement}
	\label{fig:methods}
\end{figure*}

solution strategy

\begin{algorithm}[h]
 Read data of the given problem instance\; 
 Decompose problem to subproblems.\;
 \ForEach{subproblem}{
 	 Use strategy to prepare/reduce data (e.g. filter variants, bundle flows)\;
	 Choose an algorithm for result calculation\;
	 Specify the model according to the algorithm\;
	 Fill model with data\;
	 Calculate result by applying the algorithm\;
	 Save the result for later use\;
 }
 Recompose results of subproblems to an overall result of original problem\;
 \vspace{0.2cm}
 \caption{Program orchestration for solving optimization problems}
 \label{alg:orchestration}
\end{algorithm}
